# Supplementary material for: Reconciling Model Multiplicity for Downstream Decision Making
Source: arXiv:2405.19667 source file (2024-05-30)
Supplement: Supplementary file 1 [file appendix-helper.tex]

\section{Concentration Inequalities}
\begin{theorem}[Hoeffding's Inequality \citep{Dubhashi_Panconesi_2009}] Let $X_1, \cdots, X_n$ be independent random variables bounded such that for each $i \in [n]$, $a_i \leq X_i \leq b_i$. Let $S_n = \sum_{i=1}^n X_i$ denote their sum. Then, for all $\eps > 0$, we have:
\begin{equation*}
    \Pr[\abs{S_n - \E[S_n]} \geq \eps] \leq 2 \exp\left(  \frac{-2 \eps^2}{\sum_{i=1}^n (b_i - a_i)^2} \right)
\end{equation*}
\end{theorem}

\begin{lemma} Let $\cE$ be a set of functions $\{ E : [0,1]^d \rightarrow [0,1] \}$, and let $U, V$ be any pair of random variables where $U \in [-1, 1]^d$ and $V \in [0,1]^d$. Let $D = \{ (U_1, V_1), \cdots, (U_n, V_n) \}$ be i.i.d draw of $n$ samples from $U, V$, define the Radamacher complexity of $\Pi$ by
\begin{equation*}
    \cR_n(\cE) \coloneq \E_{D, \sigma_i \sim \unif[-1,1]} \left[ \sup_{b \in B} \frac{1}{n} \sum_{i=1}^n \sigma_i b(V_i) \right]
\end{equation*}
then for any $\delta > 0$, with probability at least $1 - \delta$, for all $E \in \cE$:
\begin{equation*}
    \norm{ \frac{1}{n} \sum_{i=1}^n (U \cdot E(V)) - \E_{\cD}[U \cdot E(V)] }_2 \leq \sqrt{d} \cR_n(\cE) + \sqrt{\frac{2d}{n} \log \left(\frac{2d}{\delta} \right)}
\end{equation*}
\end{lemma}

\begin{proof}
    By norm inequality, we have:
    \begin{align*}
        \norm{\frac{1}{n} \sum_{i=1}^n (U \cdot E(V)) - \E[U \cdot E(V)]}_2 \leq \sqrt{d} \norm{\frac{1}{n} \sum_{i=1}^n (U \cdot E(V)) - \E[U \cdot E(V)]}_{\infty}
    \end{align*}

    Denote the $j-$th dimension of $U$ by $U^j$. Now, we can provide bounds for $\abs{\frac{1}{n} \sum_{i=1}^n (U^j \cdot E(V)) - \E[U^j \cdot E(V)]}$ by standard Radamacher complexity arguments. Define a set of samples $\bar{D} = \{ (\bar{U}_1, \bar{V}_1), \cdots, (\bar{U}_n, \bar{V}_n) \}$ and Radamacher variables $\sigma_i\in \{ -1, 1 \}$. We have:
    \begin{align*}
        &\E_D \left [\sup_E \abs{\frac{1}{n} \sum_{i=1}^n (U^j \cdot E(V)) - \E[U^j \cdot E(V)]} \right] \\
        &= \E_D \left[ \sup_E \abs{ \frac{1}{n} \sum_{i=1}^n (U^j \cdot E(V)) - \E_{\bar{D}} \left[ \frac{1}{n} \sum_{i=1}^n (\bar{U}^j \cdot E(\bar{V})) \right] } \right] \tag{Law of total expectation} \\
        &= \E_D \left[ \sup_{E} \abs{ \E_{\bar{\cD}} \left[ \frac{1}{n} \sum_{i=1}^n (U^j \cdot E(V)) - \frac{1}{n} \sum_{i=1}^n (\bar{U}^j \cdot E(\bar{V}))  \right] } \right] \tag{Linearity} \\
        &\leq \E_D \left[ \sup_E \E_{\bar{D}} \left[ \abs{\frac{1}{n} \sum_{i=1}^n (U^j \cdot E(V)) - \frac{1}{n} \sum_{i=1}^n (\bar{U}^j \cdot E(\bar{V}))} \right] \right] \tag{Jensen} \\
        &\leq \E_{D, \bar{D}} \left[ \sup_E \abs{\frac{1}{n} \sum_{i=1}^n (U^j \cdot E(V)) - \frac{1}{n} \sum_{i=1}^n (\bar{U}^j \cdot E(\bar{V}))} \right] \tag{Jensen} \\
        &\leq \E_{\sigma, D, \bar{D}} \left[ \sup_E \abs{\frac{1}{n} \sum_{i} \sigma_i U_i^j E(V_i) - \frac{1}{n} \sum_i \sigma_i \bar{U}_i^j E_(\bar{V}_i)} \right] \tag{Radamacher} \\
        &\leq \E_{\sigma, D, \bar{D}} \left[ \sup_E \abs{\frac{1}{n} \sum_i \sigma_i U_i^j E (V_i)} + \sup_E \abs{\frac{1}{n} \sum_i \sigma_i \bar{U}_i^j E(\bar{V}_i)} \right] \tag{Jensen} \\
        &= 2 \E_{\sigma, D} \left[ \sup_E \abs{\frac{1}{N} \sum_i \sigma_i U_i^j E(V_i)} \right]
    \end{align*}

    Suppose we know the Radamacher complexity of $\cE$. Then, by contraction inequality and $U_i^j \in [-1, 1]$, we have for any $j \in [d]$, 
    \begin{equation*}
        \cR_n(\cE) \geq \E \left[ \sup_E  \frac{1}{n} \sum_i \sigma_i U_i^j E(V_i) \right]
    \end{equation*}
    Also note that the map $D \rightarrow \frac{1}{n} \sum_i \sigma_i U_i^j E(V_i)$ has $\nicefrac{2}{n}$ bounded difference. Then, by McDiarmid's inequality, for any $\eps > 0$, we have:
    \begin{equation*}
        \Pr \left[ \sup_E \abs{\frac{1}{n} \sum_i \sigma_i U_i^j E(V_i)} \geq \cR_n (\cE) + \eps \right] \leq 2 \exp( -n \eps^2 /2)
    \end{equation*}
    Taking union bound over all coordinates $j \in [d]$, we have:
    \begin{equation*}
        \Pr \left[ \sup_j \sup_E \abs{\frac{1}{n} \sum_i \sigma_i U_i^j E(V_i)} \geq \cR_n (\cE) + \eps \right] \leq 2 d \exp( -n \eps^2 /2)
    \end{equation*}

    Combine this with norm inequality, we have:
    \begin{align*}
        &\Pr \left[ \sup_E \norm{\frac{1}{n} \sum_{i=1}^n (U \cdot E(V)) - \E[U \cdot E(V)]}_2 \geq \sqrt{d} \cR_n(\cE) + \sqrt{d} \eps \right] \\
        &\leq \Pr \left[ \max_j \sup_E  \sum_{i=1}^n (U^j \cdot E(V)) - \E[U^j \cdot E(V)] \geq \cR_n(\cE) + \eps \right]\\
        &\leq 2 d \exp (-n \eps^2 / 2)  
    \end{align*}
    Rearranging the terms, we have for all $\delta > 0$, we have:
    \begin{equation*}
        \Pr \left[ \sup_E \norm{\frac{1}{n} \sum_{i=1}^n (U \cdot E(V)) - \E[U \cdot E(V)]}_2 \geq \sqrt{d} \cR_n(\cE) + \sqrt{\frac{2d}{n} \log \left( \frac{2d}{\delta} \right)} \right] \leq \delta
    \end{equation*}
\end{proof}

\begin{lemma} Define the set:
\begin{equation*}
    \cE = \left\{ \pi_\ell^\BR(f(x)) = a, a \in [K], \ell \in \cL \right \} 
\end{equation*}
then $\cR_n(\cE) = O \left( \sqrt{\frac{d K \log(K) \log(n)}{n}} \right)$
\end{lemma}

\begin{proof}
    For all $E \in \cE$, the set $\{ f \in [0,1]^d, E_{\ell, a}(f(x), x) = 1 \}$ is the intersection of $K$ many $d$-dimensional half-planes, we have the VC-dimension of $\cE$ is: $\mathsf{VC}(\cE) \leq (d + 1) 2 K \log(3K)$. By Sauer's Lemma, we have:
    \begin{equation*}
        \cR_n(\cE) \leq \sqrt{\frac{2 \mathsf{VC}(\cE) \log(n/\mathsf{VC} (\cE) ) }{n}} = O \left( \frac{2d K \log(K) \log(n)}{n} \right) 
    \end{equation*}
\end{proof}
