# Supplementary material for: Reconciling Model Multiplicity for Downstream Decision Making
Source: arXiv:2405.19667 source file (2024-05-30)
Supplement: Supplementary file 3 [file appendix_experiment.tex]

\section{Additional Experiment Detail}
\label{appendix:experiment}

Our ImagineNet experiments are run on a Macbook Pro with $32$GB of RAM. The experiment on the ImageNet dataset uses pre-trained models provided by pyTorch, which do not require additional training. The experiment on the HAM10000 dataset includes neural network models trained using pyTorch on NVIDIA GA100 GPU ($80$ GB of RAM) with $2$ compute workers loading the data. The total time to train the two neural network models with approximately $88\%$ Top-1 accuracy takes less than $5$ minutes.
